# Supplementary material for: Learning One-hidden-layer Neural Networks with Landscape Design
Source: arXiv:1711.00501 source file (2017-11-03)
Supplement: Supplementary file 1 [file appendix-hermite.tex]

%\section{More backgrounds on Hermite Polynomials} \label{sec:backgrounds}
